# Supplementary material for: Towards Understanding Neural Collapse: The Effects of Batch Normalization and Weight Decay
Source: arXiv:2309.04644 source file (2024-09-04)
Supplement: Supplementary file 1 [file appendix_not_use.tex]

% The environment used here (theappendices) is a wrapper for the basic appendices environment which changes the appearance of the title page and the structure and appearance of the appendices in the table of contents and PDF bookmarks. The original functionality can be restored by simply removing the 'the' from the \begin{} and \end{} statements below.



\begin{comment}\section{Proof of Lemma \ref{acclemma}}
Using a similar argument as \label{interdivide}
\begin{align*}
    \text{intra}_c &= \frac{1}{N^2}\sum_{i=1}^N\sum_{j=1}^N \bar{\mathbf{h}}_{c,i}\cdot \bar{\mathbf{h}}_{c,j}\\
    &= \frac{1}{N^2}\sum_{i=1}^N\sum_{j=1}^N \frac{\mathbf{h}_{c,i}}{\|\mathbf{h}_{c,i}\|}\cdot \frac{\mathbf{h}_{c,j}}{\|\mathbf{h}_{c,j}\|}\\
    &= \frac{1}{N^2}\sum_{i=1}^N\sum_{j=1}^N \frac{\mathbf{h}_{c,i}\cdot \mathbf{h}_{c,j}}{\|\mathbf{h}_{c,i}\|\|\mathbf{h}_{c,j}\|}\\
    &= \left(\frac{1}{N}\sum_{i=1}^N \frac{\mathbf{h}_{c,i}}{\|\mathbf{h}_{c,i}\|}\right)\cdot\left(\frac{1}{N}\sum_{j=1}^N \frac{\mathbf{h}_{c,j}}{\|\mathbf{h}_{c,j}\|}\right)\\
    &= \left(\frac{1}{N}\sum_{i=1}^N \frac{\mathbf{h}_{c,i}}{\|\mathbf{h}_{c,i}\|}\right)\cdot \tilde{\bar{\mathbf{h}}}_c\\
    &= \frac{1}{N}\sum_{i=1}^N \bar{\mathbf{h}}_{c,i}\cdot \tilde{\bar{\mathbf{h}}}_c
\end{align*}
and also
\begin{align*}
    \text{inter}_c &= \frac{1}{N^2}\sum_{i=1}^N\sum_{j=1}^N \bar{\mathbf{h}}_{c,i}\cdot \bar{\mathbf{h}}_{c',j}\\
    &= \frac{1}{N^2}\sum_{i=1}^N\sum_{j=1}^N \frac{\mathbf{h}_{c,i}}{\|\mathbf{h}_{c,i}\|}\cdot \frac{\mathbf{h}_{c',j}}{\|\mathbf{h}_{c',j}\|}\\
    &= \frac{1}{N^2}\sum_{i=1}^N\sum_{j=1}^N \frac{\mathbf{h}_{c,i}\cdot \mathbf{h}_{c',j}}{\|\mathbf{h}_{c,i}\|\|\mathbf{h}_{c',j}\|}\\
    &= \left(\frac{1}{N}\sum_{i=1}^N \frac{\mathbf{h}_{c,i}}{\|\mathbf{h}_{c,i}\|}\right)\cdot\left(\frac{1}{N}\sum_{j=1}^N \frac{\mathbf{h}_{c,j}}{\|\mathbf{h}_{c',j}\|}\right)\\
    &= \left(\frac{1}{N}\sum_{i=1}^N \frac{\mathbf{h}_{c,i}}{\|\mathbf{h}_{c,i}\|}\right)\cdot \tilde{\bar{\mathbf{h}}}_{c'}\\
    &= \frac{1}{N}\sum_{i=1}^N \bar{\mathbf{h}}_{c,i}\cdot \tilde{\bar{\mathbf{h}}}_{c'}
\end{align*}
Therefore, consider random variable $i$ uniformly distributed on $[N]$, then
\begin{align*}
    \text{inter}_c &= \mathbb{E}[\bar{\mathbf{h}}_{c,i}\cdot \tilde{\bar{\mathbf{h}}}_{c'}]=1-\epsilon\\
    \text{intra}_c &= \mathbb{E}[\bar{\mathbf{h}}_{c,i}\cdot \tilde{\bar{\mathbf{h}}}_{c}]=a
\end{align*}
Also note that both $\bar{\mathbf{h}}_{c,i}\cdot \tilde{\bar{\mathbf{h}}}_{c'}$ and $\bar{\mathbf{h}}_{c,i}\cdot \tilde{\bar{\mathbf{h}}}_{c}$ is between 1 and -1. A sample $\mathbf{h}_{c,i}$ is correctly classified if $\bar{\mathbf{h}}_{c,i}\cdot \tilde{\bar{\mathbf{h}}}_{c}>\bar{\mathbf{h}}_{c,i}\cdot \tilde{\bar{\mathbf{h}}}_{c'}$. Let $X=\bar{\mathbf{h}}_{c,i}\cdot \tilde{\bar{\mathbf{h}}}_{c}$ and $Y=\tilde{\bar{\mathbf{h}}}_{c}>\bar{\mathbf{h}}_{c,i}\cdot \tilde{\bar{\mathbf{h}}}_{c'}$. Then $1-X>0$ and $1-Y>0$ 
\end{comment}
